# Supplementary material for: Anisotropic, two-dimensional, disordered Wigner solid
Source: arXiv:2207.06618 ancillary file (2022-07-14)
Supplement: Supplementary file 1 [file Supplemental_Material_two_dimensional_anisotropic_disordered_Wigner_solid.pdf]

# Supplemental Material: Anisotropic Two-Dimensional Disordered Wigner Solid

Md. S. Hossain, M. K. Ma, K. A. Villegas-Rosales, Y. J. Chung, L. N. Pfeiffer, K. W. West, K. W. Baldwin, and M. Shayegan
*Department of Electrical Engineering, Princeton University, Princeton, New Jersey 08544, USA*
(Dated: June 12, 2022)

## I. MATERIAL PLATFORM

Our material platform is an AlAs quantum well (QW) epitaxially grown via molecular beam epitaxy on a GaAs substrate. The sample contains a 21-nm-wide AlAs QW sandwiched by 68-nm $Al_{0.38}Ga_{0.62}$ barriers. Similar to the case of GaAs, as long as the conduction band offset between the barrier and the QW is sufficiently large, it is possible to confine carriers in the AlAs QW through modulation doping [1, 2]. The main difference is that in AlAs the conduction band has lower energy at the X-points of the Brillouin zone instead of the Γ-point. Therefore, the electrons in our AlAs QW are confined in the X-point valleys.

Bulk AlAs has a Zinc Blende crystal structure and it crystallizes in the cubic F-43m space group. In bulk AlAs, electrons occupy three energetically degenerate ellipsoidal (or six half-ellipsoidal) conduction-band valleys at the six equivalent X-points of the first Brillouin zone [1]. We denote these valleys as X, Y, and Z with the major axes lying along [100], [010], and [001], respectively [see Fig. S1(a)]. The electrons in each valley possess an anisotropic Fermi surface with longitudinal and transverse effective masses of $m_l = 1.1$ and $m_t = 0.20$ in units of the free electron mass [1].

When an AlAs QW is formed along the [001] axis, the confinement in the growth direction splits the three-fold valley degeneracy because of the difference in the effective mass along the in-plane and out-of-plane directions. We refer to the out-of-plane valley as Z, and the in-plane valleys as X and Y. At first sight, one would expect that the Z valley should be occupied at all well-widths since it has a larger mass along the confinement direction. However, the slightly larger lattice constant of AlAs compared to GaAs causes biaxial compression in the plane of the AlAs layer, lowering the conduction band of the X and Y valleys relative to the Z valley. This causes the ground-state energies of the two types of valleys to cross at a critical QW width of $\simeq 6$ nm [1]. Above this well-width, the X and Y valleys are occupied; this is the case for our 21-nm-wide AlAs QW [Fig. S1(b)].

In the absence of any additional in-plane strain, electrons in our AlAs QW occupy two in-plane valleys (X and Y) [Fig. S1(b)]. This two-fold valley-degeneracy is lifted as the density is lowered below $6.3\times10^{10}$ cm$^{-2}$ (see Ref. [3]for details).

Electron-beam evaporated Ti-Au alloy on the backside of the sample serves as a back gate which we use to change the 2DES density ($n$) *in situ*. Electrical contacts to the 2DES are achieved via alloying a eutectic mixture of In and Sn on the corners and the centers of the sample edges at 425 $^o$C for 270 seconds.

We carried out our experiments in a $^3$He cryostat with a base temperature of $T \simeq 0.30$ K.

## II. MEASUREMENTS OF DIFFERENTIAL RESISTANCE AS A FUNCTION OF DC BIAS

Sample response as a function of applied dc bias provides information on the $I$-$V$ characteristics of the sample. We use such measurements to probe the pinned Wigner solid (WS) phase as shown in the main text. For these measurements, we use a setup shown in Fig. S2. The dc input is taken from the lock-in amplifier and the dc current that flows through the sample is obtained via measuring the voltage drop across a known series resistance (1 kΩ) using a high-precision dc voltmeter. On the other hand, a small ac signal (0.5 nA, 1.7 Hz) is used to extract the differential resistance directly from the lock-in amplifier. Note that, we use a separate lock-in amplifier to measure $I_{ac}$; this enables us to measure large values of differential resistances ($dV/dI$).

We note that the data shown in Figs. 1(b-d) of the main text were all taken at $V_{dc} = 0$ and with an ac current excitation of 1 nA, except for the two lowest traces in Fig. 1(b) where 2 nA was used.

## III. INTERPLAY BETWEEN THE WIGNER SOLID AND QUANTUM HALL STATES

Here we comment on the interplay between the Wigner solid (WS) and quantum Hall states at very low densities. Intriguingly, in our sample, the integer and fractional quantum Hall (FQH) states, manifested by clear minima in $R_{[100]}$ at Landau level filling factors $\nu = 1$ and $1/3$, persist up to very large $r_s$ values [e.g., $r_s = 49$ and 45, see Fig. 1**b** of the main text], even when the ground state at $B = 0$ exhibits an insulating behavior with extremely large resistances and non-linear $I$-$V$ characteristics, suggestive of a disordered WS pinned by the ionized impurities. Our observation implies that a localized 2DES at $B = 0$ can make a transition to an FQH (liquid) state at large perpendicular magnetic fields. This may sound somewhat non-intuitive at first sight since high magnetic fields usually instigate transitions from a liquid to a solid instead of a solid to a liquid state. However, it is well known that there are pinned, insulating WS states that are reentrant around FQH states [4–17]. It has indeed been shown that Landau level mixing can change the boundaries (in terms of the filling factor) between the WS and FQH liquid states [11, 17, 18]. Note that the Landau level mixing parameter, typically quantified by the ratio of the Coulomb to cyclotron energies, is equal

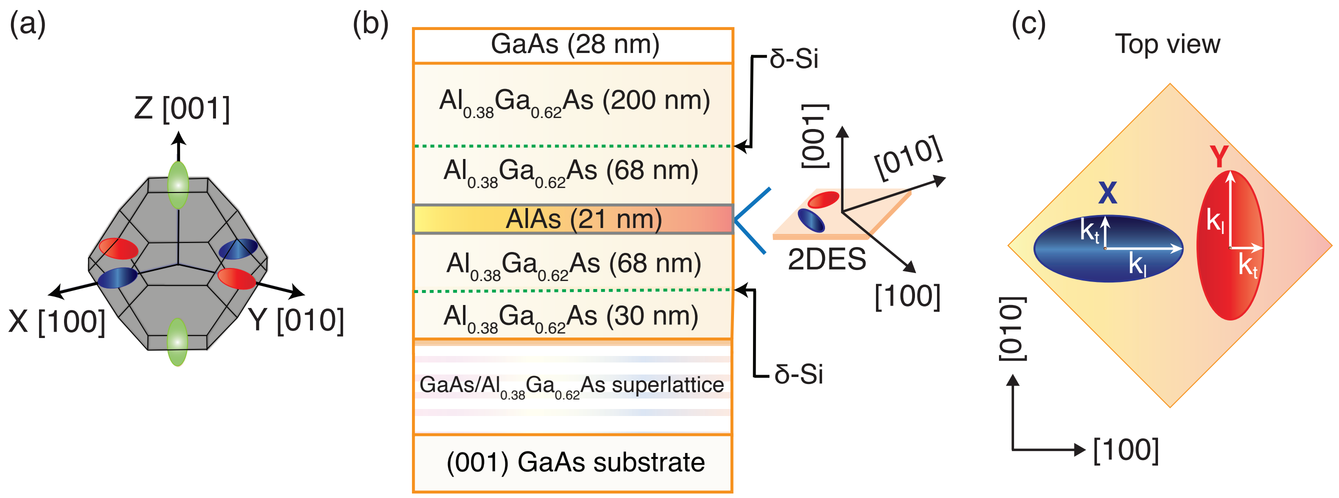


FIG. S1. (a) First Brillouin zone and constant energy surfaces of the lowest-energy bands for bulk AlAs, showing the X, Y, and Z valleys; [100], [010], and [001] refer to the crystallographic directions. (b) Structure of our AlAs 2DES grown on a GaAs substrate. The growth direction is [001]. The AlAs layer is under compressive biaxial strain because of the slightly larger lattice constant of AlAs relative to GaAs. This strain results in the occupancy of X and Y valleys only. (c) Relative orientations of the Fermi wavevectors ($k_l$ and $k_t$) of the elliptical X and Y valleys with respect to the crystallographic directions, [100] and [010]. $k_l$ ($k_t$) denotes the major (minor) axes of the two valleys. Therefore, for the X valley, $k_l$ ($k_t$) is along [100] ([010]) while for the Y valley, $k_l$ ($k_t$) is along [010] ([010]).

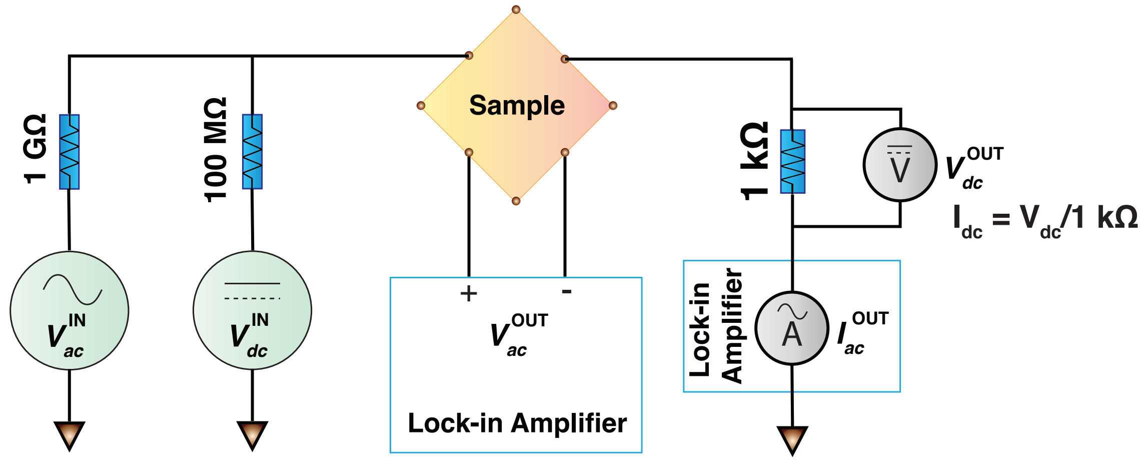


FIG. S2. Experimental setup for measuring differential resistance as a function of dc bias, showing the current injection and voltage leads used to measure both dc and ac quantities in order to obtain the $dV/dI$ vs. $I_{dc}$ ($V_{dc}$) plots.

to $(\nu/2)^{1/2} r_s$. Zhao *et al.* [18] show that, at $\nu = 1/3$, the FQH liquid state is favored over the WS even when the mixing parameter is as high as $\simeq 18$, which translates to an $r_s$ of $\simeq 44$ where a WS is expected at $B = 0$. Our experimental data lend support to this theoretical work, demonstrating that a WS at $B = 0$ can make a transition to a FQH liquid state at $\nu = 1/3$. We note, however, that in our data at very low densities, while the Hall resistances exhibit quantized plateaus at the expected values, the corresponding longitudinal resistances are $>> h/e^2$ and do not go to zero at low temperatures [15, 19]. This led to a proposal that the state we observe at $\nu = 1/3$ is not a quantum Hall liquid, but rather an exotic quantized Hall insulator [19, 20]. We would like to emphasize that, no matter what the correct interpretation of our data is, our observation of FQH features at extremely low densities (down to $n \simeq 1.2$, $r_s \simeq 45$) strongly implies that there is a significant amount of electron-electron interaction present in the low-density insulating phases that we report here.

## IV. SPIN POLARIZATION OF THE OBSERVED PINNED WIGNER SOLID

It has been theoretically predicted that an anisotropic WS can harbor antiferromagnetic spin order [21]. Our magnetotransport experiments, however, indicate that when the density

is lowered below $\simeq$ 2.0, the 2DES becomes ferromagnetic, and there is no sign that the magnetization changes at lower $n$ [15].

To elaborate, here we discuss the spin polarization data at very low electron densities. We measure magnetoresistance as a function of $B_{||}$. In Fig. S3 we show such data taken at densities ranging from $n = 2.60$ to 1.10. For the densities $n = 2.60$ and 2.10, the resistance increases with $B_{||}$ because of the loss of screening due to increasing polarization. The resistance rises until $B_{||} = B_M$ where polarization is maximized; $B_M$ is known as the magnetizing field; see Ref. [15] and references therein. As the density is lowered to $n = 2.00$, the resistance becomes independent of $B_{||}$ indicating $B_M = 0$, and thus signaling ferromagnetism, i.e., that the 2DES is already fully spin polarized at $B_{||} = 0$. This behavior stems from interaction-induced magnetization at low densities, the details of which are discussed elsewhere [15]. Notably, as seen in Fig. S3, the resistance stays flat as a function of $B_{||}$ down to the lowest density ($n = 1.10$), where the ground state is a pinned WS.

Based on the discussion above, the pinned WS that we observe appears to host ferromagnetic order instead of the theoretically predicted antiferromagnetic order. We emphasize that the magnetic order of very dilute 2DESs is very delicate as the competing states have extremely close ground state energies [22].

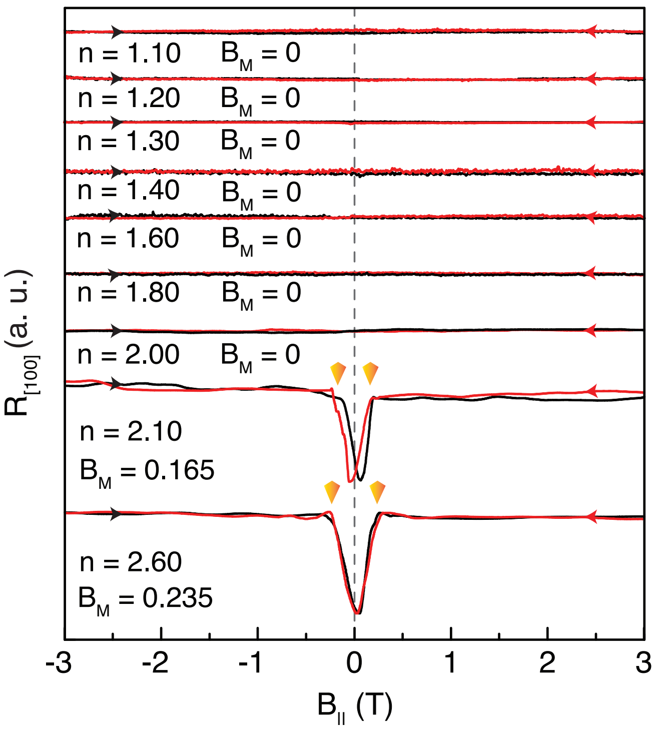


FIG. S3. The resistance along the [100] direction $R_{[100]}$, taken at $T = 0.30$ K, plotted against $B_{||}$ at different 2DES densities. Traces are shown for both up- and down-sweeps of $B_{||}$ and are offset vertically. The vertical arrows (placed symmetrically with respect to $B_{||} = 0$) mark the positions of $B_M$ above which the resistance saturates, and are based on the average of four values of $B_M$ (for up- and down-sweeps, and $+B_{||}$ and $-B_{||}$). For $n \leq 2.00$, the traces are flat and $B_M = 0$. $B_M$ stays zero even for $n \lesssim 1.80$ where the 2DES freezes into a Wigner solid, suggesting a ferromagnetic Wigner solid.

## V. DENSITY DEPENDENCE OF THE NON-LINEAR DIFFERENTIAL RESISTANCE

Here we discuss the density dependence of $dV/dI$ and its anisotropy along [100] and [010]. In Fig. 2(a) of the main text, we show $dV/dI$ vs. $V_{dc}$ data along [100] and [010] at very low densities, namely $n = 1.10$, 1.20, 1.30, and 1.50. Here we also include data at higher densities, i.e., $n = 1.70$, 1.80, 2.0, and 2.50. Figure S4 shows such data. It is clear in Fig. S4 that the non-linearity in current-voltage characteristics and the presence of sharp voltage thresholds in $dV/dI$ emerge below $n = 1.80$ which we attribute to the critical density for the WS formation. At and above $n = 1.80$, $dV/dI$ is essentially constant as a function of $V_{dc}$.

It is worthwhile noting that although the non-linearity disappears at $n \geq 1.80$, the anisotropy ($dV/dI_{[010]} > dV/dI_{[100]}$) persists, reflecting the effective mass anisotropy. However, there are differences in the nature of anisotropy between the $dV/dI$ data for $n < 1.80$ and $n \geq 1.80$. For $n < 1.80$, the anisotropy can change as a function of $V_{dc}$. Such changes are the consequence of anisotropic voltage thresholds. For instance, at a fixed density and at slightly above $V_{th[100]}$, $dV/dI_{[100]}$ drops abruptly, but $dV/dI_{[010]}$ is still pinned to its large, saturated value, leading to a rise in anisotropy. In contrast, such changes do not occur for $n \geq 1.80$, where the anisotropy is fixed as a function of the dc bias.

[1] M. Shayegan, E. P. De Poortere, O. Gunawan, Y. P. Shkolnikov, E. Tutuc, and K. Vakili, Two-dimensional electrons occupying multiple valleys in AlAs, Phys. Stat. Sol. (b) **243**, 3629 (2006).
[2] Y. J. Chung, K. A. Villegas Rosales, H. Deng, K. W. Baldwin, K. W. West, M. Shayegan, and L. N. Pfeiffer, Multivalley two-dimensional electron system in an AlAs quantum well with mobility exceeding $2 \times 10^6$ cm$^2$/Vs, Phys. Rev. Materials **2**, 071001(R) (2018).
[3] M. S. Hossain, M. K. Ma, K. A. Villegas Rosales, Y. J. Chung, L. N. Pfeiffer, K. W. West, K. W. Baldwin, and M. Shayegan, Spontaneous valley polarization of itinerant electrons, Phys. Rev. Lett. **127**, 116601 (2021).
[4] E. Y. Andrei, G. Deville, D. C. Glattli, F. I. B. Williams, E. Paris, and B. Etienne, Observation of a Magnetically Induced Wigner Solid, Phys. Rev. Lett. **60**, 2765 (1988).
[5] H. W. Jiang, R. L. Willett, H. L. Stormer, D. C. Tsui, L. N. Pfeiffer, and K. W. West, Quantum liquid versus electron solid around $\nu = 1/5$ Landau-level filling, Phys. Rev. Lett. **65**, 633 (1990).
[6] V. J. Goldman, M. Santos, M. Shayegan, and J. E. Cunningham, Evidence for two-dimentional quantum Wigner crystal, Phys. Rev. Lett. **65**, 2189 (1990).
[7] Y. P. Li, T. Sajoto, L. W. Engel, D. C. Tsui, and M. Shayegan,

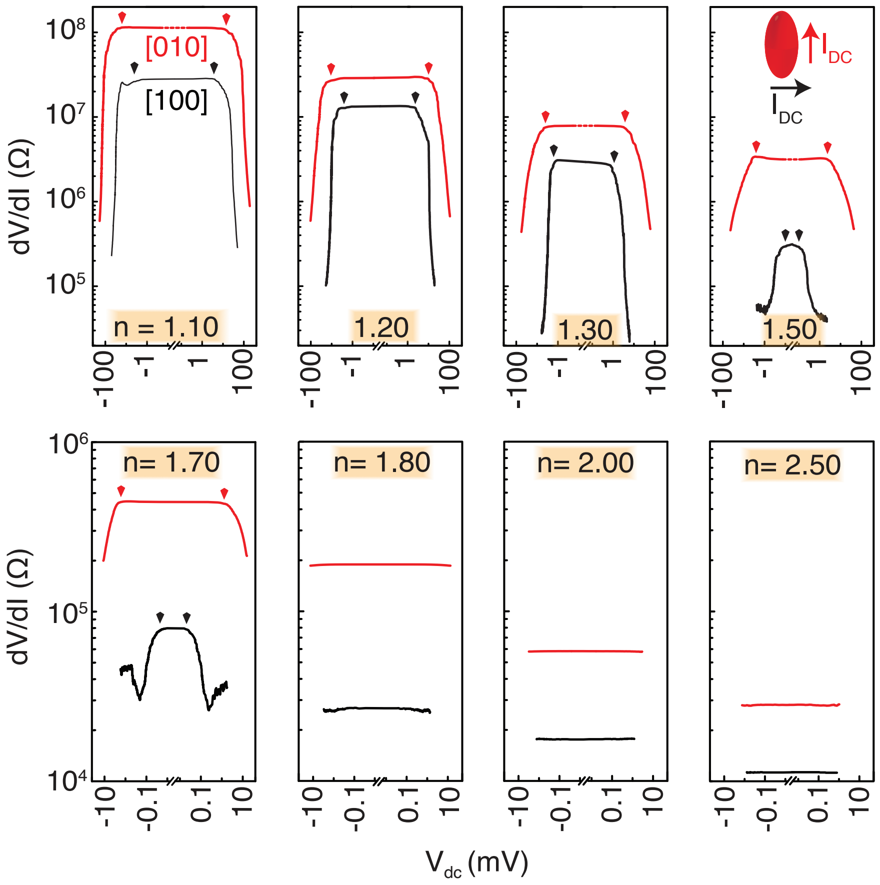


FIG. S4. $dV/dI$ data at $T = 0.30$ K along the [100] (black traces) and [010] (red traces) crystallographic directions, plotted as a function of the dc voltage drop along the sample. Data are shown for $n = 1.10$, 1.20, 1.30, 1.50, 1,70, 1.80, 2.0, and 2.50 (in units of $10^{10}$ cm$^{-2}$). Note that the $V_{dc}$ scales for the upper and lower panels are different. For $n \lesssim 1.80$, along both directions $dV/dI$ traces show a reasonably abrupt drop above a threshold voltage ($V_{th}$) which depends on the direction; $V_{th}$ is smaller for transport along [100] compared to [010]. The vertical arrows (placed symmetrically with respect to $V_{dc} = 0$) mark $V_{th}$, and are based on the average value of $V_{th}$ for $+V_{dc}$ and $-V_{dc}$. On the other hand, there is no threshold behavior seen for $n \geq 1.80$. The resistance anisotropy can still be seen for $n \geq 1.80$ reflecting the effective mass anisotropy.


M. Low-frequency noise in the reentrant insulating phase around the $1/5$ fractional quantum Hall liquid, Phys. Rev. Lett. **67**, 1630 (1991).

[8] F. I. B. Williams, P. A. Wright, R. G. Clark, E. Y. Andrei, G. Deville, D. C. Glattli, O. Probst, B. Etienne, C. Dorin, C. T. Foxon, and J. J. Harris, Conduction Threshold and Pinning Frequency of Magnetically Induced Wigner Solid, Phys. Rev. Lett. **66**, 3285 (1991).

[9] H. Buhmann, W. Joss, K. von Klitzing, I. V. Kukushkin, A. S. Plaut, G. Martinez, K. Ploog, and V. B. Timofeev, Novel magneto-optical behavior in the Wigner-solid regime, Phys. Rev. Lett. **66**, 926 (1991).

[10] E. M. Goldys, S. A. Brown, R. B. Dunford, A. G. Davies, R. Newbury, R. G. Clark, P. E. Simmonds, J. J. Harris, and C. T. Foxon, Magneto-optical probe of two-dimensional electron liquid and solid phases, Phys. Rev. B **46**, 7957 (1992).

[11] M. B. Santos, Y. W. Suen, M. Shayegan, Y. P. Li, L. W. Engel, and D. C. Tsui, Observation of a reentrant insulating phase near the 1/3 fractional quantum Hall liquid in a two-dimensional hole system, Phys. Rev. Lett. **68**, 1188 (1992).

[12] Y. P. Chen, G. Sambandamurthy, Z. H. Wang, R. M. Lewis, L. W. Engel, D. C. Tsui, P. D. Ye, L. N. Pfeiffer, and K. W. West, Melting of a 2D quantum electron solid in high magnetic field, Nat. Phys. **2**, 452 (2006).

[13] H. Deng, Y. Liu, I. Jo, L. N. Pfeiffer, K. W. West, K. W. Baldwin, and M. Shayegan, Commensurability Oscillations of Composite Fermions Induced by the Periodic Potential of a Wigner Crystal,Phys. Rev. Lett. **117**, 096601 (2016).

[14] H. Deng, L. N. Pfeiffer, K. W. West, K. W. Baldwin, L. W. Engel, and M. Shayegan, Probing the Melting of a Two-Dimensional Quantum Wigner Crystal via its Screening Efficiency, Phys. Rev. Lett. **122**, 116601 (2019).

[15] M. S. Hossain, M. K. Ma, K. A. Villegas Rosales, Y. J. Chung, L. N. Pfeiffer, K. W. West, K. W. Baldwin, and M. Shayegan, Observation of spontaneous ferromagnetism in a two-dimensional electron system, Proc. National Acad. Sci. **117**, 32244 (2020).

[16] M. K. Ma, K. A. Villegas Rosales, H. Deng, Y. J. Chung, L. N. Pfeiffer, K. W. West, K. W. Baldwin, R. Winkler, and M. Shayegan, Thermal and Quantum Melting Phase Diagrams for a Magnetic-Field-Induced Wigner Solid, Phys. Rev. Lett. **125**, 036601 (2020).

[17] K. A. Villegas Rosales, S. K. Singh, Meng K. Ma, Md. Shafayat Hossain, Y. J. Chung, L. N. Pfeiffer, K. W. West, K. W. Bald-

win, and M. Shayegan, Competition between fractional quantum Hall liquid and Wigner solid at small fillings: Role of layer thickness and Landau level mixing, Phys. Rev. Research **3**, 013181 (2021).

[18] J. Zhao, Y. Zhang, and J. K. Jain, Crystallization in the fractional quantum Hall regime induced by Landau-level mixing, Phys. Rev. Lett. **121**, 116802 (2018).

[19] Kyung-Su Kim, Steven A. Kivelson, Discovery of an insulating ferromagnetic phase of electrons in two dimensions, Proc. National Acad. Sci. **118**, e2023964118 (2021).

[20] D. Shahar, D. C. Tsui, M. Shayegan, J. E. Cunningham, E. Shimshoni, S. L. Sondhi, On the nature of the Hall insulator. Solid State Commun. **102**, 817 (1997).

[21] C. Zhou and R. N. Bhatt, Zero temperature magnetic phase diagram of Wigner crystal in anisotropic two-dimensional electron systems, Physica B: Condensed Matter **403**, 1547 (2008).

[22] N. D. Drummond and R. J. Needs, Phase Diagram of the Low-Density Two-Dimensional Homogeneous Electron Gas, Phys. Rev. Lett. **102**, 126402 (2009).
